# Supplementary material for: Towards Accurate Reconstruction of 3D Scene Shape from A Single Monocular Image
Source: arXiv:2208.13241 source file (2022-09-04)
Supplement: Supplementary file 1 [file A1.tex]

\begin{figure}[t]   
\centering
\includegraphics[width=\linewidth]{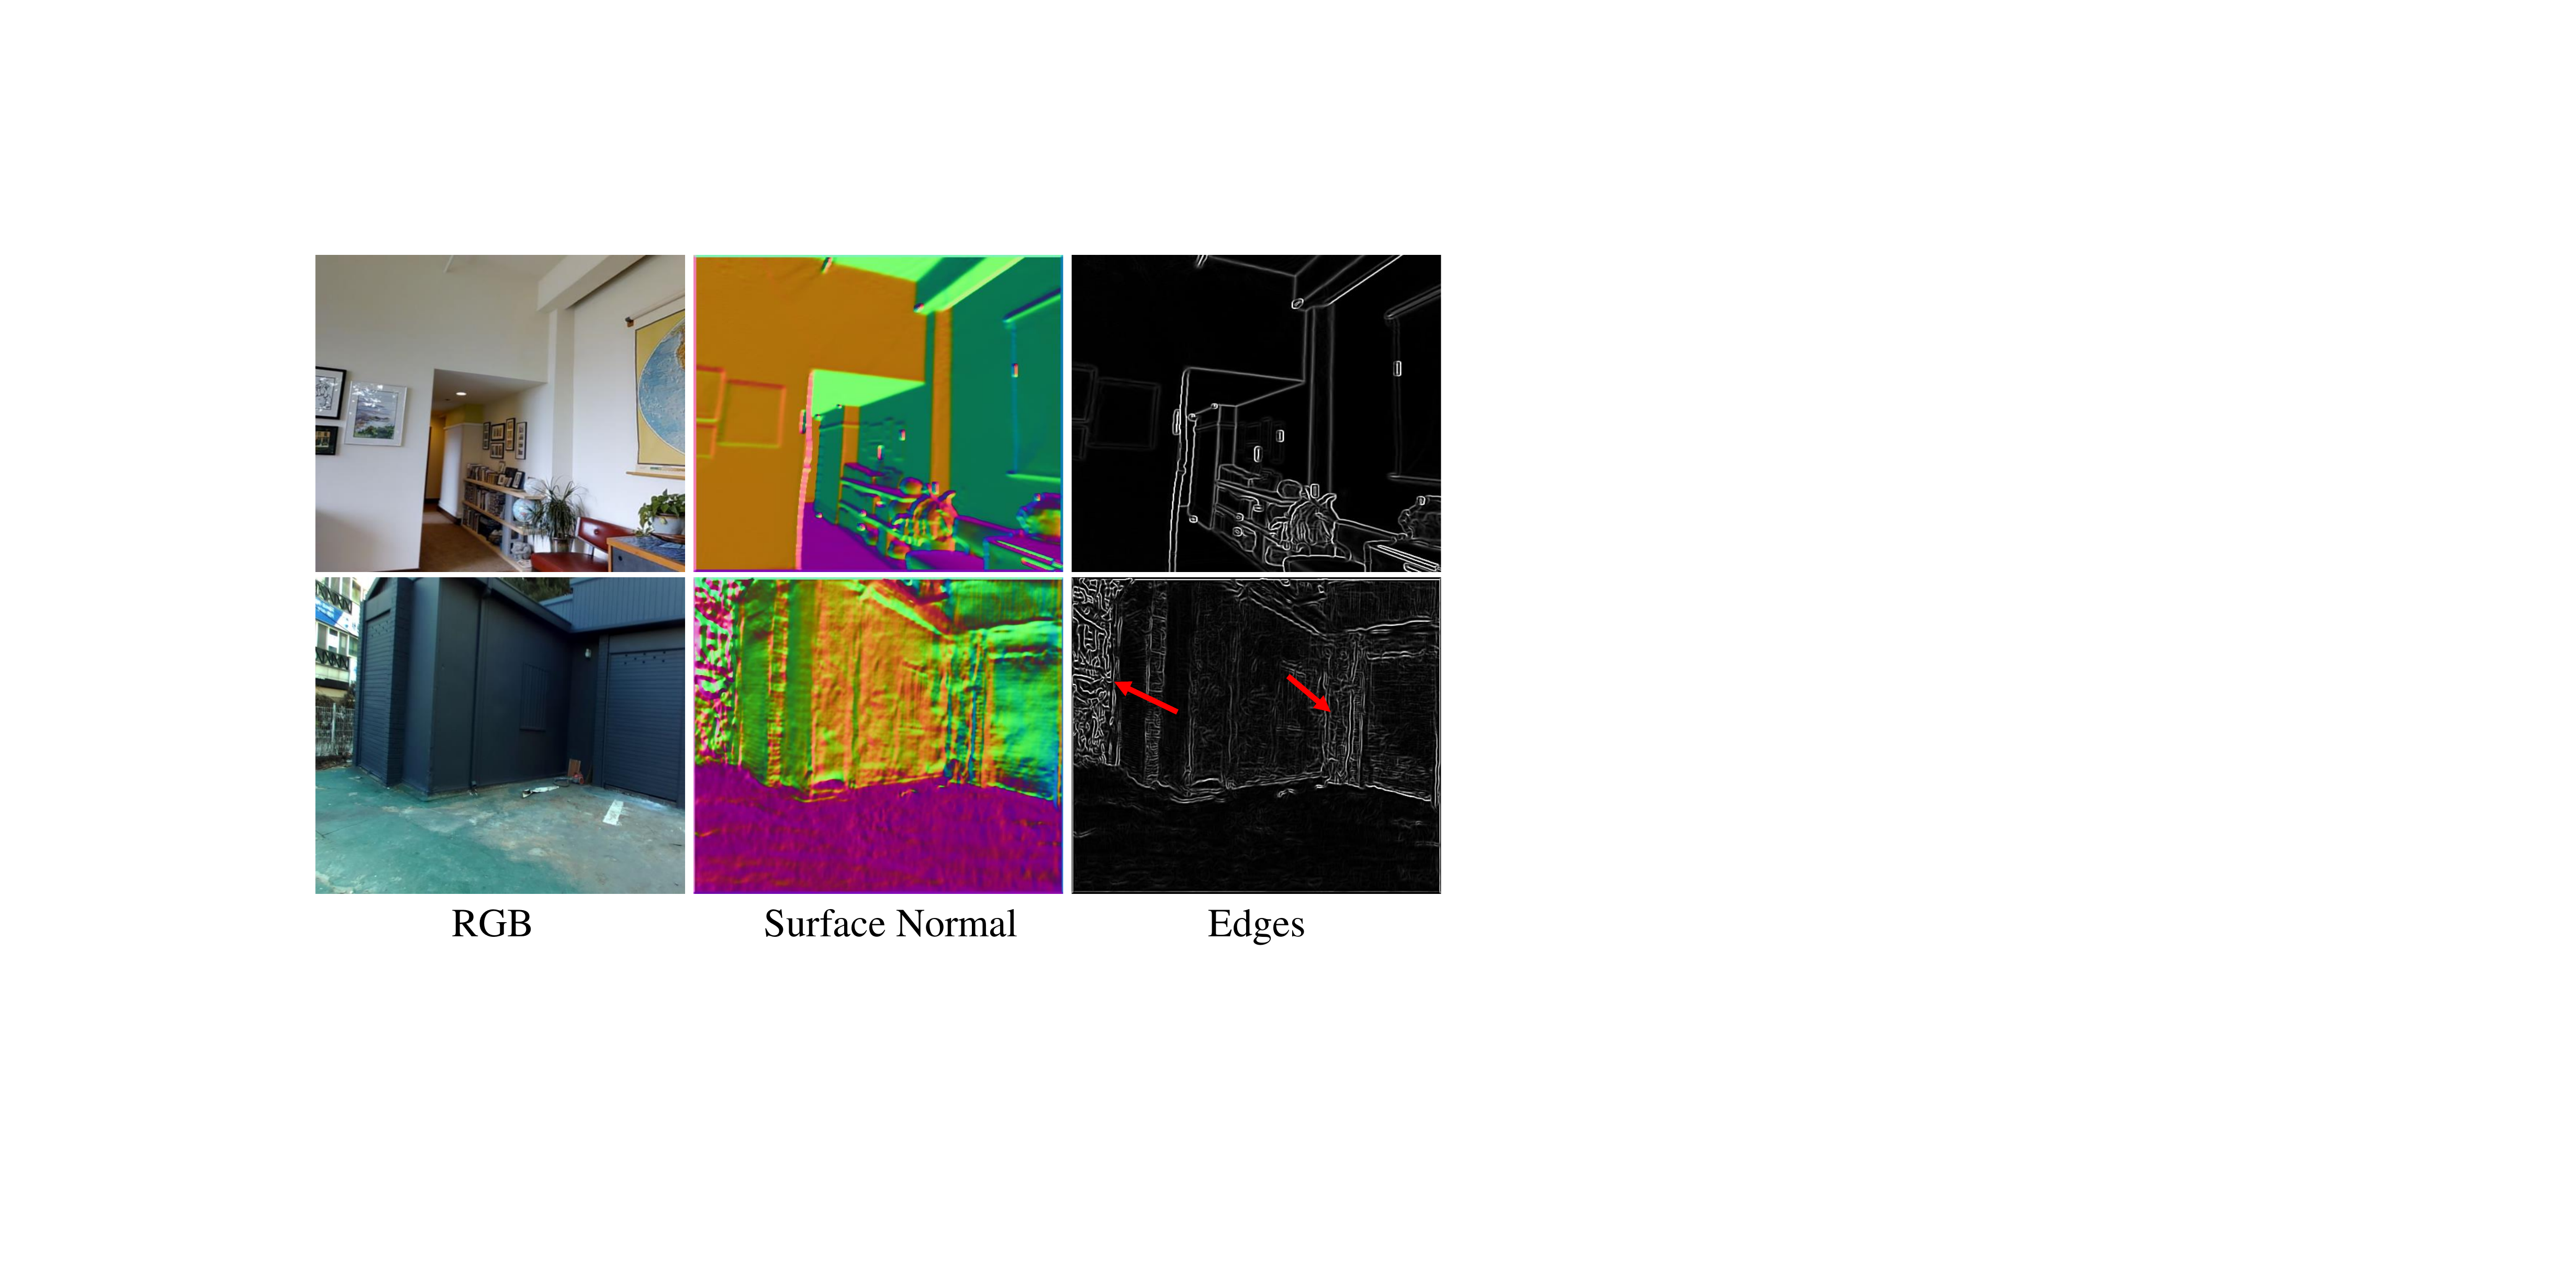}
\caption{Detected edges on high-quality (Taskonomy~\cite{zamir2018taskonomy}, the first row) and middle-quality data (DIML~\cite{kim2018deep}, the second row). There are more artifacts on DIML (see red arrows). }
%\vspace{-0.5em}
\label{Fig: cmp of edges.}
\end{figure}
