# Supplementary material for: Towards Accurate Reconstruction of 3D Scene Shape from A Single Monocular Image
Source: arXiv:2208.13241 source file (2022-09-04)
Supplement: Supplementary file 4 [file A7.tex]

\begin{figure*}[ht]
\centering
\includegraphics[width=.75\linewidth]{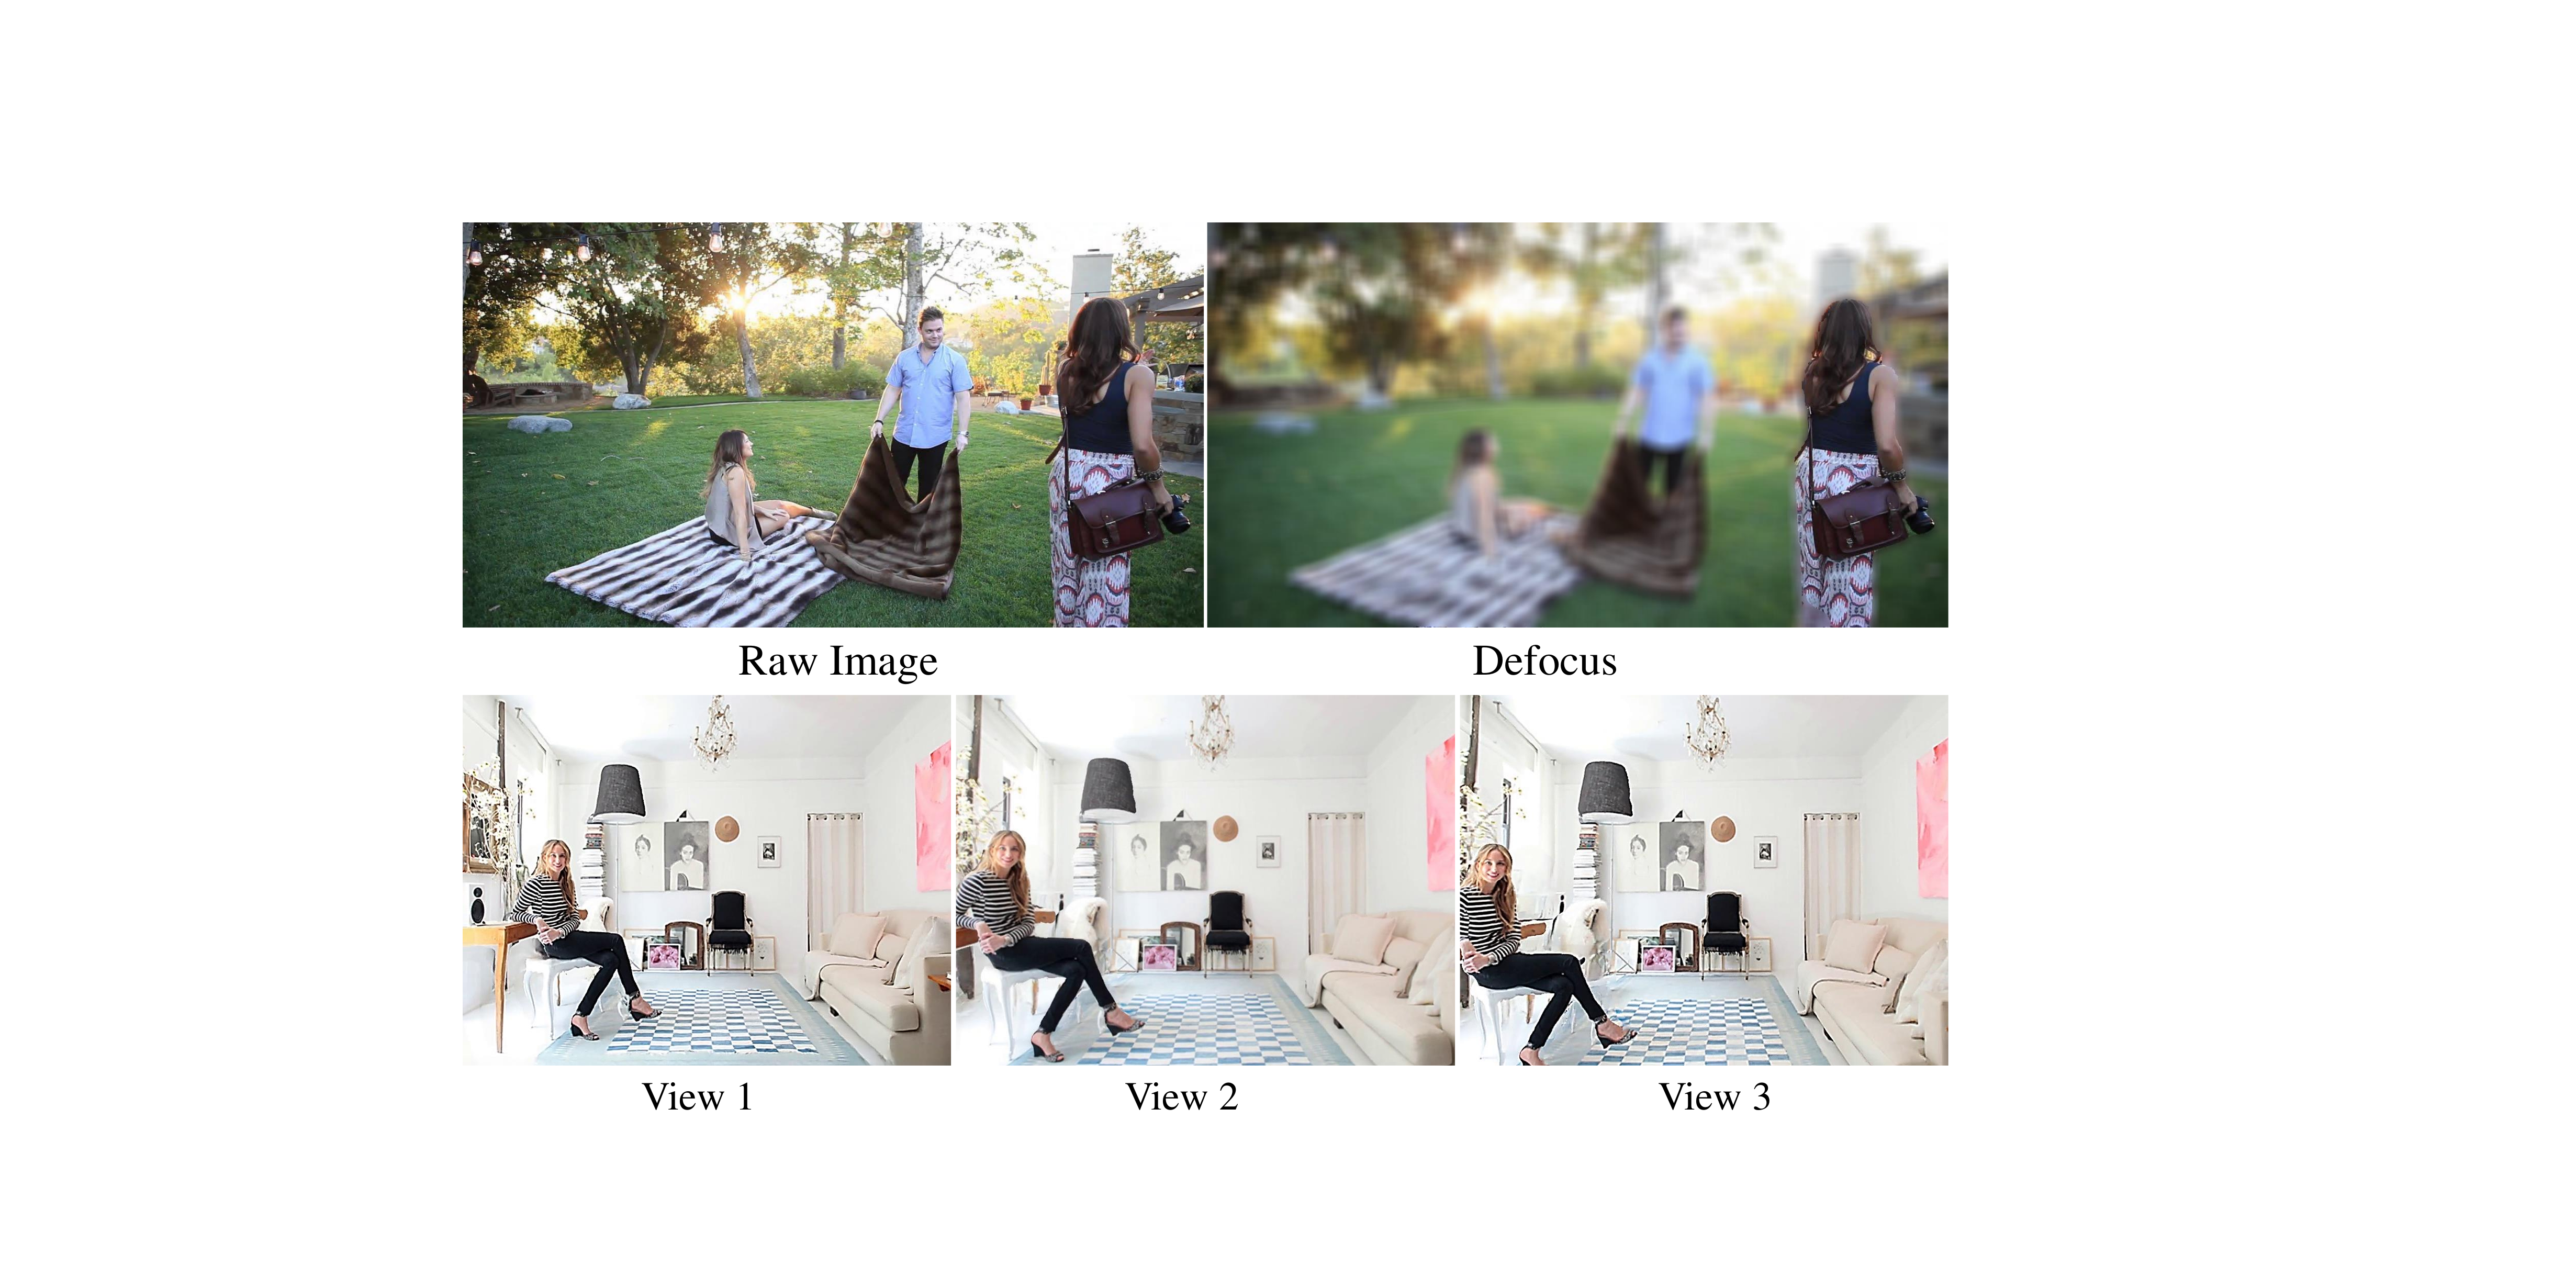}
\caption{
% Qualitative 
\textcolor{black}{\textbf{Illustration of some applications}. We 
%employ
use 
our predicted depth to create some visual effects on a single input image. The first row %is
shows results of 
defocused images, while the second row is an example of new views synthesis.}}
\label{Fig: cmp of 3D photo. }
%\vspace{-1 em}
\end{figure*}
